# Supplementary material for: OMG-ATTACK: Self-Supervised On-Manifold Generation of Transferable Evasion Attacks
Source: arXiv:2310.03707 source file (2023-10-05)
Supplement: Supplementary file 1 [file 99_appendix.tex]

\section{Experimental Setting Details}
\label{apx:exp_settings}

Tables \ref{tab:mnist_hyperparameters}, \ref{tab:traffic_hyperparameters} , \ref{tab:birds_hyperparameters} shows the evaluated models' hyperparameters per dataset.

\begin{table}[ht]
\centering
\begin{tabularx}{\linewidth}{Xr}
\toprule
\textbf{Module} & \textbf{\# Parameters} \\ 
\midrule
Generator & 1.8M \\
Discriminator & 1.6M \\
\mnisttgt{} & 694K \\ 
\mnisttra{} & 629K \\ 
\mnisttrb{} & 893K \\ 
Resnet18 & 11.1M \\ 
\midrule
\textbf{Hyperparameter} & \textbf{Value} \\ 
\midrule
Batch Size & 256 \\ 
Max Optimization Steps & 15,000 \\
Encoder Loss Update Frequency & 2 \\ 
Embedding Dimension & 128 \\ 
Temperature & 0.1 \\  
Contrastive Loss Weight & 1 \\ 
Budget & 0.3 \\ 
Generator Loss Update Frequency & 1 \\ 
Generator Learning Rate & 0.0001 \\ 
Generator Optimizer & Adam \\ 
Generator Weight Decay & 0 \\
On Manifold Loss Weight & 10 \\ 
Contrastive Loss Weight & 2 \\  
Discriminator Learning Rate & 0.0001 \\ 
\bottomrule
\end{tabularx}
\caption{Hyperparameters and the number of parameters per module used in training the \ofirmodel{} on the MNIST dataset.}
\label{tab:mnist_hyperparameters}
\end{table}

\begin{table}[h]
\centering
\begin{tabularx}{\linewidth}{Xr}
\toprule
\textbf{Module} & \textbf{\# Parameters} \\ 
\midrule
Generator & 1.8M \\
Discriminator & 1.6M \\
STN-CNN & 855K \\ 
Resnet50 & 23.6M \\ 
\midrule
\textbf{Hyperparameter} & \textbf{Value} \\ 
\midrule
Batch Size & 128 \\ 
Max Optimization Steps & 100,000 \\
Encoder Loss Update Frequency & 1 \\ 
Embedding Dimension & 350 \\ 
Temperature & 0.1 \\  
Contrastive Loss Weight & 1 \\ 
Budget & 0.015 \\ 
Generator Loss Update Frequency & 1 \\ 
Generator Learning Rate & 0.0001 \\ 
Generator Optimizer & Adam \\ 
Generator Weight Decay & 0 \\
On Manifold Loss Weight & 5 \\ 
Contrastive Loss Weight & 5 \\  
Discriminator Learning Rate & 0.0001 \\ 
\bottomrule
\end{tabularx}
\caption{Hyperparameters and the number of parameters per module used in training the \ofirmodel{} on the GTSRB dataset.}
\label{tab:traffic_hyperparameters}
\end{table}
\begin{table}[h]
\centering
\begin{tabularx}{\linewidth}{Xr}
\toprule
\textbf{Module Name} & \textbf{\# Parameters} \\ 
\midrule
Generator & 1.8M \\
Discriminator & 2.8M \\
Resnet18 & 11.3M \\ 
Resnet50 & 23.9M \\ 
Resnet50W & 67.2M \\ 
\midrule
\textbf{Hyperparameter} & \textbf{Value} \\ 
\midrule
Batch Size & 24 \\ 
Max Optimization Steps & 60,000 \\
Encoder Loss Update Frequency & 1 \\ 
Embedding Dimension & 2,048 \\ 
Temperature & 0.1 \\  
Contrastive Loss Weight & 1 \\ 
Budget & 0.025 \\ 
Generator Loss Update Frequency & 2 \\ 
Generator Learning Rate & 0.0001 \\ 
Generator Optimizer & Adam \\ 
Generator Weight Decay & 0 \\
On Manifold Loss Weight & 10 \\ 
Contrastive Loss Weight & 2 \\  
Discriminator Learning Rate & 0.0001 \\ 
\bottomrule
\end{tabularx}
\caption{Hyperparameters and the number of parameters per module used in training the \ofirmodel{} on the \birds{} dataset.}
\label{tab:birds_hyperparameters}
\end{table}

\section{Qualitative Results}
\label{apx:vis_results}

A showcase of adversarial examples generated by the \ofirmodel{} model for the various datasets, can be found in the Supplementary Material..

% \input{omg-attack-arow23/tables/apx_birds_examples}
% \input{omg-attack-arow23/tables/apx_traffic_examples}

% \input{omg-attack-arow23/tables/apx_birds_examples}
% \input{omg-attack-arow23/tables/apx_traffic_examples}

% \begin{figure*}
%   \centering
%   \includegraphics[width=0.8\textwidth]{omg-attack-arow23/figures/mnist_showcase-01-02-02.png}
%   \caption{Evasion Attacks on MNIST dataset representative, on the left we have the original image, then the EAs using FGSM, then the diff. On the right side, we have the same paradigm for EAs generated using \ofirmodel{} model.\adi{remove?}}
%   \label{fig:mnist_showcase}
% \end{figure*}
